# Supplementary material for: Self-stratifying turbidity currents
Source: arXiv:2207.13826 source file (2023-03-03)
Supplement: Supplementary file 1 [file SteadyState.tex]

\section{Steady Flow}

In this section we report the steady versions of \cref{eqn:1Dsys_vol_DE,eqn:1Dsys_part_DE,eqn:1Dsys_mom_DE,eqn:1Dsys_egy_DE} rearranged as evolution equations for $h$, $\Fro$, $\beta$, and $\gamma$. The denominator of the system is
\begin{multline} \label{eqn:system_denominator}
	\mathcal{D} 
	\eqdef 16 w_s^3 \sigma_{uu}^2 \sigma_{z\phi} \sigma_{u\phi} h \gamma^3 
	\Bigg(
		\sigma_{uu} \sigma_{z\phi} \ppar*{ 2 \sigma_{uk} - \beta \sigma_{uk}'} \Fro^2 \ppar*{ \Fro^2 - 1 }
	\\
		+ \beta \gamma^2 \Bigg[
			\sigma_{z\phi} \sigma_{uuu} \ppar*{2 \frac{\sigma_{uu}'}{\sigma_{uu}} - \frac{\sigma_{uuu}'}{\sigma_{uuu}}} \Fro^4 
		%\\
			+ \sigma_{z\phi} \sigma_{uuu} \ppar*{- \frac{\sigma_{u\phi}'}{\sigma_{u\phi}} + \frac{\sigma_{uuu}'}{\sigma_{uuu}} + \frac{\sigma_{z\phi}'}{\sigma_{z\phi}}} \Fro^2
		\\
			+ \sigma_{uu} \varsigma_{zu\phi} \ppar*{+ 2 \frac{ \sigma_{u\phi}' }{ \sigma_{u\phi} } -2 \frac{ \sigma_{uu}' }{ \sigma_{uu} } -2 \frac{ \varsigma_{zu\phi}' }{ \varsigma_{zu\phi} } } \Fro^2
		%\\
			+ \varsigma_{zu\phi} \sigma_{uu} \ppar*{ - \frac{\sigma_{u\phi}'}{\sigma_{u\phi}} + 2 \frac{\varsigma_{zu\phi}'}{\varsigma_{zu\phi}} - \frac{\sigma_{z\phi}'}{\sigma_{z\phi}} }
		\Bigg]
	\Bigg)
\end{multline}
where primes represent differentiation with respect to $\beta$. For similarity flow 
\begin{align}\label{eqn:system_denominator_similarity}
	\mathcal{D} 
	= 32 w_s^3 \sigma_{uu}^3 \sigma_{z\phi}^2 \sigma_{u\phi} \sigma_{uk} h \gamma^3 \Fro^2 \ppar*{ \Fro^2 - 1 }
\end{align}
and consequently the system becomes singular when $\Fro \in \{-1,0,1\}$. The governing equations are
\begin{multline}
	\mathcal{D} \dv{h}{x}
	= 4 D \sqrt{2} \sigma_{uu}^{\frac{5}{2}} \beta  \gamma^{2} h w_s^{2} \sigma_{z\phi} 
	\Bigg(
		2 \sigma_{uk} \sigma_{u\phi} \sigma_{uu} \sigma_{z\phi} \Fro^2 \pbrk*{ 4 \Fro^2 - 1 }
	\\
		+ 2 \Fro^{4} \beta \gamma^{2} \sigma_{u\phi} \sigma_{uuu} \sigma_{z\phi} \pbrk*{ 3 \frac{\sigma_{uu}'}{\sigma_{uu}} - 2 \frac{\sigma_{uuu}'}{\sigma_{uuu}} }
	%\\
		+ 2 \Fro^{4} \beta \sigma_{uk} \sigma_{u\phi} \sigma_{uu} \sigma_{z\phi} \pbrk*{ \frac{\sigma_{uu}'}{\sigma_{uu}} - 2 \frac{\sigma_{uk}'} {\sigma_{uk}} }
	\\
		+ \Fro^{2} \beta  \gamma^{2} \sigma_{u\phi} \sigma_{uuu} \sigma_{z\phi} \pbrk*{ -3 \frac{\sigma_{u\phi}'}{\sigma_{u\phi}} + \frac{\sigma_{uuu}'}{\sigma_{uuu}} + 3 \frac{\sigma_{z\phi}'}{\sigma_{z\phi}} }
	\\
		+ \Fro^{2} \beta \sigma_{uk} \sigma_{u\phi} \sigma_{uu} \sigma_{z\phi} \pbrk*{ \frac{\sigma_{uk}'}{\sigma_{uk}} - \frac{\sigma_{u\phi}'}{\sigma_{u\phi}} + \frac{\sigma_{z\phi}'}{\sigma_{z\phi}} }
	\\
		+ 2 \beta  \gamma^{2} \sigma_{u\phi} \sigma_{uu} \varsigma_{zu\phi} \pbrk*{ \frac{\sigma_{u\phi}'}{\sigma_{u\phi}} - \frac{\varsigma_{zu\phi}'}{\varsigma_{zu\phi}} } \pbrk{4 \Fro^2 - 1}
	\Bigg) S_h
\\
	+ 2 D^{3} \Fro^{2} \sqrt{2} \sigma_{uu}^{\frac{5}{2}} R \beta^{3} g h^{2} \sigma_{z\phi} \Bigg(
		2 \sigma_{uk} \sigma_{uu} \sigma_{z\phi}^{2} \Fro^{2}
	\\
		+ \pbrk*{4 \sigma_{uu}' \varsigma_{zu\phi} \sigma_{z\phi} \gamma^{2} - \sigma_{uuu}' \sigma_{z\phi}^{2} \gamma^{2} - \sigma_{uk}' \sigma_{uu} \sigma_{z\phi}^{2} } \beta \Fro^{2}
	\\
		+ 2 \beta  \gamma^{2} \sigma_{z\phi} \sigma_{uu} \varsigma_{zu\phi} \pbrk*{ \frac{\sigma_{z\phi}'}{\sigma_{z\phi}} - \frac{\varsigma_{zu\phi}'}{\varsigma_{zu\phi}} }
	\Bigg) S_\Phi
\\
	+ 8 \sigma_{z\phi} D^{2} \beta^{2} h \gamma \Fro^{2} w_s \sigma_{uu}^{2} \Bigg(
		-2 \sigma_{uk} \sigma_{u\phi} \sigma_{uu} \sigma_{z\phi} \Fro^{2}
	\\
		+ \sigma_{u\phi} \sigma_{z\phi} \pbrk*{ \sigma_{uuu}' \gamma^{2} + \sigma_{uk}' \sigma_{uu} } \beta \Fro^{2}
	%\\
		+ 2 \varsigma_{zu\phi} \sigma_{u\phi} \sigma_{uu} \pbrk*{ \frac{\varsigma_{zu\phi}'}{\varsigma_{zu\phi}} - \frac{\sigma_{u\phi}'}{\sigma_{u\phi}} } \beta  \gamma^{2}
	\Bigg) S_U
\\
	- 4 D^{3} \Fro^{2} \sqrt{2} \sigma_{uu}^{\frac{7}{2}} \beta^{4} \gamma^{2} h \sigma_{z\phi} \sigma_{u\phi} \Bigg( 2 \Fro^{2} \frac{\sigma_{uu}'}{\sigma_{uu}} - \frac{\sigma_{u\phi}'}{\sigma_{u\phi}} + \frac{\sigma_{z\phi}'}{\sigma_{z\phi}} \Bigg) S_T
\end{multline}

\note{is it worth typesetting the other 3 equations? They're all this bad...}
